# Supplementary material for: From Chaotic Spin Dynamics to Non-collinear Spin Textures in YIG Nano-films by Spin Current Injection
Source: arXiv:2009.10628 source file (2020-09-22)
Supplement: Supplementary file 1 [file SupplementaryInformation.pdf]

# Supplementary Information

Henning Ulrichs*

*I. Physical Institute, Georg-August University of Göttingen,*

*Friedrich-Hund-Platz 1, 37077 Göttingen, Germany*

(Dated: September 18, 2020)

## Abstract

In this supplement, I first explain details about data generation and processing. Then, I discuss the effect of the Oersted field induced by the charge current in the Pt stripe. Afterwards, I present simulations of a YIG film with significantly larger damping, in order to connect the micromagnetic modeling to experimental work. Then, a brief analysis of the non-thermal spectral properties developing at large, spatially unrestricted current densities is shown. I end with a short comment on the Reynolds number in the injection region.

## DETAILS ON DATA GENERATION AND DATA PROCESSING

The data shown in Figure 2, 3 and 4 in the main article refer to individual time series with a length of 70 ns, from which only the last 50 ns were considered for Fast Fourier transformation (FFT) and for the computation of $\Psi$ and $\Sigma$. For the computing the data shown in Figure 5, time series with a length of 20 ns were considered. Regarding $\Sigma$, one can understand why this quantity is proportional the number of emitted magnons, when recalling that classically [1], for a sample magnetized along $x$-direction, the magnon occupation number $n$ is proportional to the square of the transversal magnetic components, which fluctuate dynamically:

$$n \propto M_y^2 + M_z^2 = M_0^2 - M_x^2. \tag{S1}$$

The last equality holds, because the modulus of the $\mathbf{M} = M_0$ is conserved. Recall that, in the micromagnetic simulation a coarse graining procedure is applied to include thermal effects: A part of thermally activated magnons is expressed implicitly via a reduction of $M_0$ in each simulation cell, while the larger wave number fluctuations are explicetly simulated. Note that, the magnons giving rise to the reduction of the $M_0$ have frequencies $\omega/2\pi = \frac{k_B T}{h} \approx 6\,\mathrm{THz}$ in the THz-range, and are partially already on the optical branches of the complex magnon spectrum of YIG [2]. While such so-called thermal modes certainly contribute to spin transport phenomena, their occupation number $n$ is hardly affected by the spin current in the experimental situation considered here. For thermal magnons one finds that, their frequency is about $2\pi\omega = \frac{k_B T}{h} \approx 6\,\mathrm{THz}$, and therefore the dissipation rate $\omega_R \approx \alpha\omega \gg \beta(j) \approx \alpha 2\pi f_0$. One can then estimate [3]

$$n = \frac{k_B T}{\hbar\omega}\frac{\omega_R}{\omega_R - \beta(j)} \approx \frac{k_B T}{\hbar\omega}. \tag{S2}$$

To get rid of the explicitly simulated part of the thermal background not related to the spin injection, $\Sigma$, as defined in Equation 5 in the main article, includes a subtraction of this contribution. By considering the not normalized vector component $M_x$, the implicitly described part of the thermal background is also removed from $\Sigma$.

The data shown in Figure 5 refers to a time series of 2d maps $m_z(x, y)$ with a length of 35 ns, equidistantly saved all 5 ps, from which the last 10 ns were used for Fourier transformations. In particular, for the 2d spatial FFT power maps $P_{\mathrm{FFT}}\{m_z(x,\, y)\}(k_x, k_y)$

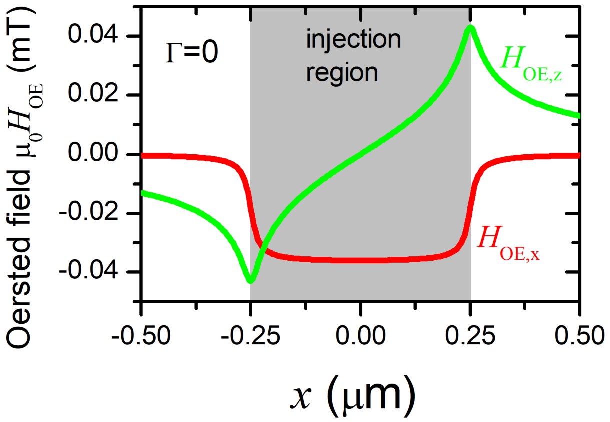


Figure 1. Oersted field inside the YIG film. Analytical calculation assuming a current density of $0.17 \cdot 10^{11}$A/m$^2$.

(left panels in Figure 5), an average over all 2d maps was computed. For the spatio-temporal FFT maps $P_{\mathrm{FFT}}(k_x, f)_{k_y=0}$ shown in the right panel of Figure 5, sections at $k_y = 0$ through each spatial 2d FFT power map were used to perform the temperoral FFT.

Note that, for all data shown in the main article and here, extensive testing regarding initialization, and the length of initial transients were carried out. Thereby it is assured that, all analysis performed afterwards with the obtained data refers to dynamic equilibrium states.

## CONFINMENT EFFECTS

The current density in the Pt injection stripe gives rise to a surrounding Oersted field $H_{oe}(x)$. The total field inside the YIG film is then inhomogeneous. Note that, when the damping is compensated by the spin torque, the current flow direction necessary for this case then gives rise to an antiparallel configuration of $H_{oe}$ with respect to the external field. If the arising potential well is strong, one can expect that, the dynamics underneath the Pt stripe is trapped in this region. To justify, why I have neglected the Oersted field in the main article, I here supply a calculation of the internal field. To calculate $H_{oe}(x)$ I have used analytical formulas,[4] derived from applying the Biot-Savart law to the case of an infinite wire with rectangular cross section (3.5 nm×500 nm).

At the threshold current density for the onset of bullet formation of $0.17 \cdot 10^{11}$A/m$^2$,

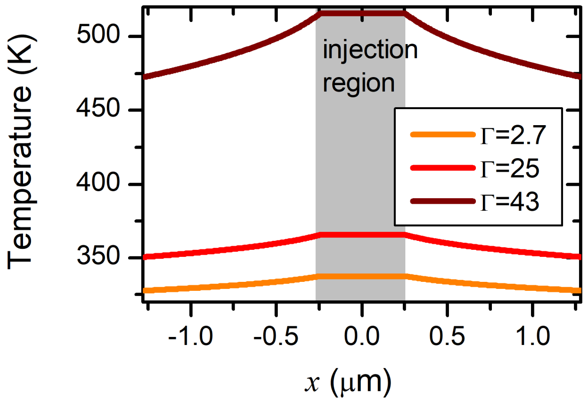


Figure 2. Temperature profile $T(x)$ inside the YIG film for different overcriticalites $\Gamma$ as indicated.

the Oersted field has a size of only about 0.036$,mT underneath the Pt stripe, as Figure 1 shows. This smallness is related to the fact that the Pt film is very thin, and therefore a rather small absolute current flows through the film (at the threshold only 0.02975 mA). Even for the largest current densities appearing in this work of $8.5 \cdot 10^{11}\,\mathrm{A/m^2}$, the typical size of the Oersted field does not exceed 1.6 mT. Considering the external field of $50\,mT$, the Oersted field cause only a rather shallow potential well.

In addition to the Oersted field, also lateral inhomogeneity of the temperature $T(x)$ may give rise to a confinement effect, due to the induced inhomogeneity of magnetic properties $M_0(x)$ and $A(x)$. In particular, since Gadolinium Gallium Garnet, which is the typically used substrate for YIG films, is an insulator with a rather low thermal conductivity of about 7 W/mK, heat generated in the Pt stripe diffuses very slowly away from the injection region.

Figure 2 shows the approximate stationary profile $T(x)$ inside the YIG film, estimated using finite element modelling. At the threshold current density $j_{th}$ ($\Gamma = 0$) the system remains everywhere rather far away from the Curie temperature of the YIG film. Therefore, the induced inhomogeneity of the magnetic material parameters remains small. At significant overcriticality $\Gamma$, the lateral inhomogeneity is instead quite pronounced, as Figure 3 shows.

Figure 4 presents snapshots of simulations taking into acount both, the presence of the Oersted field, as well as lateral profiles $M_0(x)$ and $A(x)$, due to inhomogeneous temperature $T(x)$. Note that, also the magnitude of the thermal field is adapted locally according to $T(x)$. Close to the threshold current density, the smallness of the Oersted field and of the temperature induced inhomogeneities in $M_0$ and $A$ explain, why no change in the magnetic

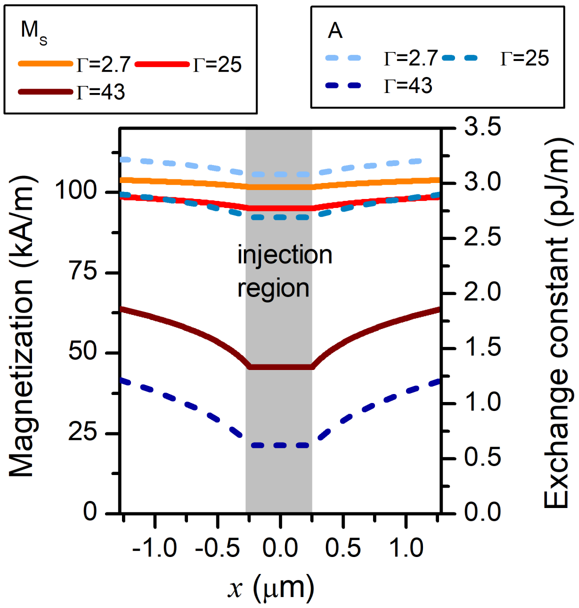


Figure 3. Profiles of magnetic parameters due to inhomogeneous temperature $T(x)$ inside the YIG film for different overcriticalites $\Gamma$ as indicated.

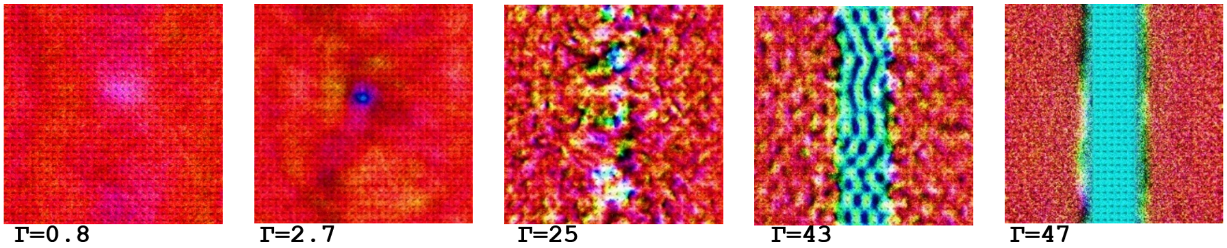


Figure 4. Simulation results including the Oersted field and inhomogenous temperature $T(x)$. Snapshots of the magnetization for different overcriticalites $\Gamma$ as indicated. Same color code as used in the main article in Figure 2.

dynamics in simulations incorporating these effects arise. But even at much larger current densities, when at least the inhomogeneity of the material parameters is significant, I could not find a qualitiative change compared to simulations neglecting these effects.

## RELATION TO EXPERIMENTAL WORK

To connect the simulation with experimental work, one has to acknowledge that, nano-sized YIG films as used in [5, 6] often display a significant so-called inhomogeneous linewidth

contribution $\Delta H(T)$ to the magnetic dissipation, which is caused by morphological and magnetic inhomogeneity. This contribution can in principle also be included in a micromagnetic simulation by modeling a realistic microstructure. The advantage of such an approach is that two-magnon scattering into modes with large wave numbers [7] is correctly included. Regarding magnon-mediated spin transport, these exchange modes for sure contribute to measured transport properties. On the other hand, for interpretation of experimental data shown in references [5, 6], a much simpler phenomenological approach is successfully applied. Accordingly, one can assume a field-dependent modification of the effective Gilbert damping by setting

$$\alpha_{eff} = \alpha + \alpha_{sp} + \frac{\gamma\mu_0 \Delta H(T)}{2\omega_0(T)}, \tag{S3}$$

where $\omega_0(T) = \sqrt{\omega_H(\omega_H + \gamma\mu_0 M(T))}$. To simulate the 13.4 nm thin YIG film from reference [6], I have assumed $\alpha + \alpha_{sp} = 0.008$, and $\Delta H = 3.6$ mT. Figure 5(a) to (d) show snapshots of the normalized magnetization $m$ at different overcriticalities. Qualitatively, the dynamics looks quite similar to the dynamics found with small damping (see Fig. 2 (a) to (f) in the main article).

In summary, the simulation of a YIG film with enlarged damping yields a larger threshold for the onset of bullet formation, as to be expected. The onset again fits quite well to the theoretical expectation of $2.63(7) \cdot 10^{11}$ A/m$^2$ (green dashed line in Fig. 5(e)), computed from solving $\beta(j) = \alpha_{eff}\,(\omega_H + 0.5\gamma\mu_0 M(j))$ for $j$. In addition, the value agrees very well with the lower threshold of $2.7(1)\cdot 10^{11}$ A/m$^2$ reported in [6]. Note that, the second threshold reported in [6] at $3.31(6)\cdot 10^{11}$ A/m$^2$, is there related to the appearance of a so-called swasing state [8]. Regarding the simulation results shown here, the second threshold of $5.3(5) \cdot 10^{11}$ A/m$^2$ (blue dashed vertical line in Fig. 5(e)) is here related to the onset of condensation of the quasi-static texture.

Furthermore, conducting a similar simulation with sample and material parameters reported in reference [5] allows to reproduce the threshold related there to the onset of non-linear spin conductance. From the simulation I have found that, this onset coincides with the appearance of spin-wave bullets.

## CHARACTERIZATION OF THE MAGNONIC TURBULENCE

In particular for the case of unrestricted spin-current injection, chaotic dynamics appeared over a wide range of overcriticality. Here, I suggest to characterize this strongly excited state by means of a Fourier analysis of the magnetization in a single simulation cell at the center of the simulated area. Figure 6(a) shows a Fourier power spectrum $P_{FFT}(f)\{m_y^c(t)\}$ for $\Gamma = -1$ , that is without spin current injection. Note that, since the raw spectrum is rather noisy, I smoothed the data as a guide to the eye. A double logarithmic plot enables a simple linear fitting (dashed line in Fig. 6(a)), yielding an exponent for a power law. The spectrum decays linearly with a slope (exponent) of $-0.9$ in the frequency range above the FMR peak at $f_0 = 2.7\,\text{GHz}$ up to $100\,\text{GHz}$. Such a slope is close to the expected value of $-1$ for a thermally activated, classical two dimensional wave system with quadratic dispersion. When increasing the charge current $j$, and therefore the temperature, but switching of the action of the spin current, the spectra do not change qualitatively (see Fig. 6(b) to (d)). This is also reflected by the fitted slope, which stays at about $-0.9$ for all overcriticalities (see Fig. 6(e)). The presence of a spin current in contrast obviously drives the subthermal magnons out of thermal equilibrium, as the spectrum in Fig. 6(b) corresponding to $\Gamma = 6.4$ shows (brown line). The slope is now about $-2.26(1)$.

At $\Gamma = 21$ (see Fig. 6(c)), the spectrum looks similar with a slightly larger slope of about $-1.863(2)$ . A more striking difference is that, the gap in the fluctuation spectrum has vanished. This implies that the mode softening discussed in relation with Fig. 3 (c) in the main article has completely occurred in this case. Indeed, at $\Gamma = 39$ (see Fig. 6(d)), the fluctuations are in magnitude below the thermal agitation level for frequencies above $10\,\text{GHz}$. Interestingly, above $\Gamma = 30$, where the onset of the condensation into the quasi-static texture was found, the slope suddenly drops, indicating an efficient suppression of small wavelength fluctuations. This is in agreement with the suppression of magnon emission outside of the actively excited area, observed in the case of confined spin-current injection (see Fig. 4 in the main article and related discussion). The evolution of the dynamics is further summarized in Fig. 6(f), where the integrated Fourier power

$$F = \int_0^{0.5\,\text{THz}} df P_{FFT}(f)\{m_y^c(t)\} \tag{S4}$$

is shown as a function of the overcriticality. When considering Joule heating alone, this

quantity simply grows monotonously (blue data points in Fig. 6(f)). With spin current included, one sees a quick initial growth up to a maximum at $\Gamma = 6.4$, where a plateau is reached. Note that, the fact that, no decrease of $F$ at large $\Gamma$ can be seen does not contradict the observed suppression of magnon emission discussed above. The reason is that, the significant spectral weight below $f_0$ is related to spin-wave modes existing only inside the actively excited area, since radiation is spectrally forbidden.

In hydrodynamic theory, a typical quantity to characterize a flow is the Reynolds number $Re$. While it is beyond my scope to estimate the latter out of the simulations, I can here at least provide an argument, why in case of strong spin current injection, one should expect large $Re$. Quite recently, Ulloa et al. [9] found for YIG films

$$Re \propto \frac{\tau_m}{\tau_{mm}}, \tag{S5}$$

which is the ratio between relaxation rates due to magnon- and momentum-conserving processes $1/\tau_{mm}$, and momentum-nonconserving processes $1/\tau_m$. Considering the injection region, the spin-transfer torque effectively compensates the latter, giving rise to very large $Re$, or with other words to a turbulent flow.

* hulrich@gwdg.de

[1] H. Suhl, Journal of Physics and Chemistry of Solids **1**, 209 (1957).

[2] A. J. Princep, R. A. Ewings, S. Ward, S. Tóth, C. Dubs, D. Prabhakaran, and A. T. Boothroyd, npj Quantum Materials **2**, 63 (2017).

[3] V. E. Demidov, S. Urazhdin, E. R. J. Edwards, M. D. Stiles, R. D. McMichael, and S. O. Demokritov, Phys. Rev. Lett. **107**, 107204 (2011).

[4] https://www.ntmdt-si.com/resources/spm-theory/theoretical-background-of-spm/2-scanning-force-microscopy-(sfm)/27-magnetic-force-microscopy-quantitative-results-treatment/279-magnetic-field-of-rectangular-conductor-with current,.

[5] N. Thiery, A. Draveny, V. V. Naletov, L. Vila, J. P. Attané, C. Beigné, G. de Loubens, M. Viret, N. Beaulieu, J. Ben Youssef, V. E. Demidov, S. O. Demokritov, A. N. Slavin, V. S. Tiberkevich, A. Anane, P. Bortolotti, V. Cros, and O. Klein, Phys. Rev. B **97**, 060409 (2018).

[6] T. Wimmer, M. Althammer, L. Liensberger, N. Vlietstra, S. Geprägs, M. Weiler, R. Gross, and H. Huebl, Phys. Rev. Lett. **123**, 257201 (2019).

[7] M. Sparks, R. Loudon, and C. Kittel, Phys. Rev. **122**, 791 (1961).

[8] S. A. Bender, R. A. Duine, A. Brataas, and Y. Tserkovnyak, Phys. Rev. B **90**, 094409 (2014).

[9] C. Ulloa, A. Tomadin, J. Shan, M. Polini, B. J. van Wees, and R. A. Duine, Phys. Rev. Lett. **123**, 117203 (2019).

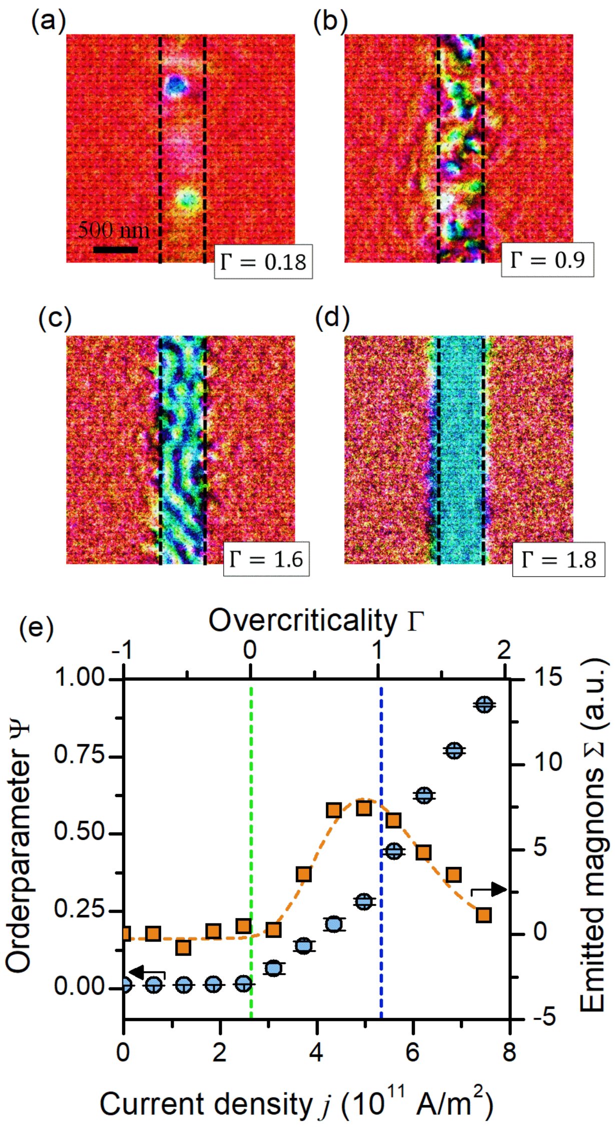


Figure 5. Spin-current induced dynamics in a YIG nano-film with increased damping. (a) to (d) Snapshots of $m$ at different current densities and thus different overcriticalities $\Gamma$ as indicated. Same color-code as in Fig. 2 in the main article. (e) Dependence of the order parameter $\Psi$ (blue circles) and of the magnon emission $\Sigma$ (orange rectangles) on the current density $j$, for the case of large damping due to sample inhomogeneity. The horizontal green dashed line marks the theoretically estimated onset of bullet formation. The blue dashed lines marks the emergence of the quasi-static texture. Orange dashed line is a guide to the eye.

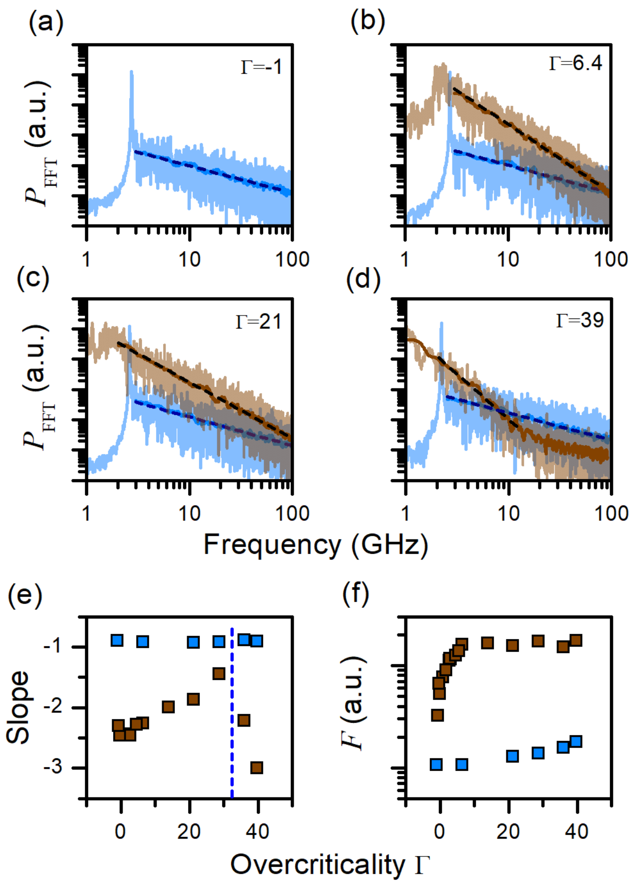


Figure 6. Evolution of magnetic fluctuations at large overcriticalities. (a) to (d) show Fourier power spectra generated by Joule heating only (light blue) and by the combined action of Joule heating and spin currents (light brown) at $\Gamma$ as indicated. Dark blue and brown lines are corresponding smoothed spectra, dashed lines are linear fits. (e) Dependence of fitted slopes, and in (f) of the integrated power $F$ on $\Gamma$. In (e) and (f) brown rectangles refer to the case with heating and spin currents, blue rectangles to the case of only considering Joule heating.
